# Supplementary material for: The Zero Turbulence Manifold in Fusion Plasmas
Source: arXiv:1207.4419 source file (2012-07-18)
Supplement: Supplementary file 1 [file thesis-appendix.tex]

\mypart{Appendix}
%\chapter{A Brief Description of the GS2 Algorithm}
\chapter{A Linear Test of the Implementation of Flow Shear in GS2}
\section{Introduction} 

A sheared slab transformation\cite{roberts1965gravitational} is used to derive an eigenvalue problem for the ITG mode which can then be solved numerically.

\section{The Slab Limit}

Starting with the gyrokinetic equation in toroidal geometry

\begin{verbatim}
-- to do 
\end{verbatim}

taking the limit of low Mach but steep velocity gradients

\begin{verbatim}
-- to do 
\end{verbatim}

and moving to slab geometry where: 

\begin{eqnarray}
\vct{u_0} = u_0 \frac{x}{l_u}\uv{y}
\end{eqnarray}

the following equation emerges:

\begin{eqnarray}
\nonumber \pdt{h_s} + v\pa^{'}\ub\cdot\nabla h_s + u_0\frac{x}{l_u} \pd{h_s}{y} + \vct{V_D} \cdot\nabla h_s \\ 
\nonumber + \frac{c}{B_0} \lbr \gyroRs{\chi}, h_s \rbr - \lp \pdt{h_s} \rp_c = \\
\nonumber \frac{c}{B_0}\lsq \frac{1}{L_n} + \lp \frac{\varepsilon_{s}^{'}}{T_{0s}} -\frac{2}{3} \rp \frac{1}{L_T} + 2\frac{u_0v\pa^{'}}{v_{ths}^2} \frac{B_{0t}}{B_{0p}} \frac{1}{L_u} \rsq F_{0s} \pd{\gyroRs{\chi}}{y} \\
+ \frac{e_s}{T_{0s}} \lp \pdt{\gyroRs{\chi}} + u_0\frac{x}{l_u} \pd{\gyroRs{\chi}}{y}\rp F_{0s} 
\end{eqnarray}

On moving to the linear collisionless limit, and specifying

\begin{eqnarray}
\vct{B_0} = B_0 \lp \uv{z} + \frac{x}{L_S}\uv{y} \rp \\
\end{eqnarray}

so that the magnetic drifts are small, the equation becomes: 

\begin{eqnarray}
\nonumber \pdt{h_s} + v\pa^{'}\ub\cdot\nabla h_s + u_0\frac{x}{l_u} \pd{h_s}{y} =\\ 
\nonumber \frac{c}{B_0}\lsq \frac{1}{L_n} + \lp \frac{\varepsilon_{s}^{'}}{T_{0s}} -\frac{2}{3} \rp \frac{1}{L_T} + 2\frac{u_0v\pa^{'}}{v_{ths}^2} \frac{B_{0t}}{B_{0p}} \frac{1}{L_u} \rsq F_{0s} \pd{\gyroRs{\chi}}{y} \\
+ \frac{e_s}{T_{0s}} \lp \pdt{\gyroRs{\chi}} + u_0\frac{x}{l_u} \pd{\gyroRs{\chi}}{y}\rp F_{0s} 
\end{eqnarray}

In the low Mach limit, the energy coordinate:

\begin{eqnarray}
\varepsilon_{s}^{'} \-\- to\ do
\end{eqnarray}

becomes

\begin{eqnarray}
\varepsilon_{s}^{'} = \frac{m_s \lp v\pa^{'2} + v\pp^{'2}\rp}{2}
\end{eqnarray}

and in the electrostatic limit: 

\begin{eqnarray}
\chi \rightarrow \varphi
\end{eqnarray}

so that the gyrokinetic equation becomes

\begin{eqnarray}
\nonumber \pdt{h_s} + v\pa^{'}\ub\cdot\nabla h_s + u_0\frac{x}{l_u}\pd{h_s}{y} =\\ 
\nonumber \frac{c}{B_0}\lsq \frac{1}{L_n} + \lp \frac{m_s \lp v\pa^{'2} + v\pp^{'2}\rp}{2T_{0s}} -\frac{2}{3} \rp \frac{1}{L_T} \right.\\
\nonumber \left. + 2\frac{u_0v\pa^{'}}{v_{ths}^2} \frac{B_{0t}}{B_{0p}} \frac{1}{L_u} \rsq F_{0s} \pd{\gyroRs{\varphi}}{y} \\
+ \frac{e_s}{T_{0s}} \lp \pdt{\gyroRs{\varphi}} + u_0\frac{x}{l_u} \pd{\gyroRs{\varphi}}{y}\rp F_{0s} 
\end{eqnarray}

\section{The Flying Slab Transform}

In its current form the equation has an explicit dependence on \(x\), the radial coordinate, and so cannot have solutions periodic in this direction. However, it is possible to transform to a sheared coordinate system in a moving frame where this dependence is removed:\cite{roberts1965gravitational}.

\begin{eqnarray}
z^{'} = z + u_f t\\
y^{'} = y - \frac{xz^{'}}{L_S}\\
x^{'}=x
\end{eqnarray}

Fourier modes in this new coordinate system: 

\begin{eqnarray}
\label{fouriermode}
\tilde{\varphi} \lp k_x^{'}, k_y^{'}, z^{'} \rp e^{\I  k_x^{'} x^{'} + \I k_y^{'} y^{'} + \gamma^{'} t^{'}}
\end{eqnarray}

are actually twisted shearing modes in Cartesian coordinates in the lab frame: 

\begin{eqnarray}
\tilde{\varphi} \lp k_x^{'}, k_y^{'}, z \rp e^{\I k_x^{'} x + \I k_y^{'} \lp y - \frac{xz}{L_S} - \frac{x u_f t}{L_S}\rp + \gamma^{'} t}
\end{eqnarray}

Rearranging, it can be seen that the speed \(u_f\) is the speed at which the velocity shear and the magnetic shear cancel each other to give a moving mode whose radial wavenumber does not evolve in time:

\begin{eqnarray}
\tilde{\varphi} \lp k_x^{'}, k_y^{'}, z \rp e^{\I \lsq k_x^{'} - \frac{k_y }{L_S}\lp z + u_f t  \rp \rsq x + \I k_y^{'}  y  + \gamma^{'} t}
\end{eqnarray}

In this new coordinate system:

\begin{eqnarray}
\pdt{} = u_f \pd{}{z^{'}} + u_f \frac{x}{L_S}\pd{}{y^{'}} + \pd{}{t^{'}}\\
\pd{}{x} = - \frac{z}{L_S}\pd{}{y^{'}} + \pd{}{x^{'}}\\
\pd{}{y} = \pd{}{y^{'}}   \\
\pd{}{z} =  - \frac{x}{L_S}\pd{}{y^{'}}+ \pd{}{z^{'}}  \\
\ub \cdot\nabla =  \pd{}{z^{'}} 
\end{eqnarray}

and the equation is

\begin{eqnarray}
\nonumber \pdt{h_s} + \lp v\pa^{'} + u_f \rp \pd{h_s}{z^{'}} =\\ 
\nonumber \frac{c}{B_0}\lsq \frac{1}{L_n} + \lp \frac{m_s \lp v\pa^{'2} + v\pp^{'2}\rp}{2T_{0s}} -\frac{2}{3} \rp \frac{1}{L_T} \right.\\
\nonumber \left. + 2\frac{u_fv\pa^{'}}{v_{ths}^2} \frac{B_{0t}}{B_{0p}} \frac{1}{L_S} \rsq F_{0s} \pd{\gyroRs{\varphi}}{y^{'}} \\
+ \frac{e_s}{T_{0s}} \lp \pdt{\gyroRs{\varphi}} + u_f \pd{\gyroRs{\varphi}}{z^{'}}\rp F_{0s} 
\end{eqnarray}

Since the rest of the derivation is in the transformed frame, the primes are now supressed. Applying a Fourier transform in \(x\) and \(y\) according to \eqref{fouriermode}:

\begin{eqnarray}
\nonumber \gamma h_s + \lp v\pa^{'} + u_f \rp \pd{h_s}{z} =\\ 
\nonumber \frac{\I k_y c}{B_0}\lsq \frac{1}{L_n} + \lp \frac{m_s \lp v\pa^{'2} + v\pp^{'2}\rp}{2T_{0s}} -\frac{2}{3} \rp \frac{1}{L_T} \right.\\
\nonumber \left. + 2\frac{u_fv\pa^{'}}{v_{ths}^2} \frac{B_{0t}}{B_{0p}} \frac{1}{L_S} \rsq F_{0s} J_0 \lp \frac{v\pp k\pp}{\OOs} \rp \hat{\varphi} \\
+ \frac{e_s}{T_{0s}} \lp J_0 \lp \frac{v\pp k\pp}{\OOs} \rp \pdt{\hat{\varphi}} + u_f \pd{J_0 \lp \frac{v\pp k\pp}{\OOs} \rp\hat{\varphi}}{z}\rp F_{0s} 
\end{eqnarray}

Where the gyroaverage of \(\varphi\)

\begin{eqnarray}
\gyroRs{\varphi} = \frac{1}{2\pi}\int\limits^{\pi}_{0}d\vartheta \left. \varphi  \lp \vct{r} \rp \right|_{\vct{R_s}} \\
\nonumber = \frac{1}{2\pi}\int\limits^{\pi}_{0}d\vartheta \left. \varphi  \lp \vct{R_s} + \frac{\ub \times \vct{v^{'}}}{\Omega_{0s}} \rp \right|_{\vct{R_s}} \\ 
\nonumber = \frac{1}{2\pi}\int\limits^{\pi}_{0}d\vartheta \hat{\varphi}  \exp \lbr \I k_x \lsq R_x -\frac{v_y}{\OOs} \rsq \right. \\ 
\nonumber \left.\left. + \I k_y \lsq R_y -\frac{1}{\OOs}\lp -v_x +\frac{z}{l_B} v_y \rp \rsq + \gamma^{'} t \rbr\right|_{\vct{R_s}} \\
\nonumber = \hat{\varphi}  \exp \lsq  \I k_x R_x  + \I k_y  R_y  + \gamma^{'} t \rsq \\
\nonumber \frac{1}{2\pi}\int\limits^{\pi}_{0}d\vartheta \exp \lbr - \I \frac{1}{\OOs}  \lsq  k_x v_y  + k_y \lp -v_x +\frac{z}{l_B} v_y\rp \rsq \rbr \\
\nonumber = \hat{\varphi}  \exp \lsq  \I k_x R_x  + \I k_y  R_y  + \gamma^{'} t \rsq \\
\nonumber \frac{1}{2\pi}\int\limits^{\pi}_{0}d\vartheta  \exp \lbr - \I \frac{v\pp}{\OOs}  \lsq  \lp k_x + \frac{z}{l_B} k_y  \rp\cos \vartheta  - k_y \sin\vartheta \rsq \rbr \\
\nonumber = \hat{\varphi}  \exp \lsq  \I k_x R_x  + \I k_y  R_y  + \gamma^{'} t \rsq J_0 \lp \frac{v\pp k\pp}{\OOs} \rp
\end{eqnarray}

where

\begin{eqnarray}
k\pp^2 =  \lp k_x + \frac{z}{l_B} k_y  \rp^2 + k_y^2
\end{eqnarray}

\section{Derivation of the Eigenvalue Problem}

To solve for \(h_s\), use an integrating factor:

\begin{eqnarray}
\exp \lsq \frac{\gamma^{'}}{u_f + v\pa^{'}} z \rsq 
\end{eqnarray}

so that 

\begin{eqnarray}
\nonumber \lp v\pa^{'} + u_f \rp  \pd{\hat{h_s} \exp \lsq \frac{\gamma^{'}}{u_f + v\pa^{'}} z \rsq }{z} = \exp \lsq \frac{\gamma^{'}}{u_f + v\pa^{'}} z \rsq 
\\ 
\nonumber \lbr \frac{\I k_y c}{B_0}\lsq \frac{1}{L_n} + \lp \frac{m_s \lp v\pa^{'2} + v\pp^{'2}\rp}{2T_{0s}} -\frac{2}{3} \rp \frac{1}{L_T} \right.\right. \\
\nonumber \left. + 2\frac{u_fv\pa^{'}}{v_{ths}^2} \frac{B_{0t}}{B_{0p}} \frac{1}{L_S} \rsq F_{0s} J_0 \lp \frac{v\pp k\pp}{\OOs} \rp \hat{\varphi} \\
\left. + \frac{e_s}{T_{0s}} \lp J_0 \lp \frac{v\pp k\pp}{\OOs} \rp \pdt{\hat{\varphi}} + u_f \pd{J_0 \lp \frac{v\pp k\pp}{\OOs} \rp\hat{\varphi}}{z}\rp F_{0s} \rbr
\end{eqnarray}

and integrate over \(z\), so that

\begin{eqnarray}
\label{hs_nocauchy}
\nonumber \hat{h_s} = 
\\
\nonumber \lp \left. \int\limits_{-\infty}^{z} d \tilde{z} \right|_{u_f + v\pa > 0} + \left. \int\limits_{\infty}^{z} d \tilde{z} \right|_{u_f + v\pa < 0} \rp  \exp \lsq \frac{\gamma^{'}\lp \tilde{z} - z \rp}{u_f + v\pa^{'}}  \rsq 
\\ 
\nonumber \frac{1}{u_f + v\pa^{'}} \lbr \frac{\I k_y c}{B_0}\lsq \frac{1}{L_n} + \lp \frac{m_s \lp v\pa^{'2} + v\pp^{'2}\rp}{2T_{0s}} -\frac{2}{3} \rp \frac{1}{L_T} \right.\right. \\
\nonumber \left. + 2\frac{u_fv\pa^{'}}{v_{ths}^2} \frac{B_{0t}}{B_{0p}} \frac{1}{L_S} \rsq F_{0s} J_0 \lp \frac{v\pp k\pp}{\OOs} \rp \hat{\varphi} \\
\left. + \frac{e_s}{T_{0s}} \lp J_0 \lp \frac{v\pp k\pp}{\OOs} \rp \pdt{\hat{\varphi}} + u_f \pd{J_0 \lp \frac{v\pp k\pp}{\OOs} \rp\hat{\varphi}}{z}\rp F_{0s} \rbr
\end{eqnarray}

using zero boundary conditions at \(z = \pm\infty\).

Let us now rewrite the term:

\begin{eqnarray}
\exp \lsq \frac{\gamma^{'}\lp \tilde{z} - z \rp}{u_f + v\pa^{'}} \rsq 
\end{eqnarray}

using a Cauchy integral representation:

\begin{eqnarray}
\frac{1}{2\pi \I} \intmii dk\pa \lsq k\pa - \frac{\I \gamma^{'}}{u_f + v\pa^{'}} \rsq^{-1} \exp \lsq - \I k\pa  \lp \tilde{z} - z \rp \rsq
\end{eqnarray}

The contour is closed in the upper half plane for \(\tilde{z}<z\) and in the lower half plane for \(\tilde{z}>z\). Since there is only a pole in the upper half plane for \(u_f + v\pa^{'} > 0\) and only a pole in the lower half for \(u_f + v\pa^{'} < 0\) the conditions on \(u_f + v\pa^{'}\) in \eqref{hs_nocauchy} can be dropped.

This means that the \(k\pa\) integrals combined with the integrals from \eqref{hs_nocauchy} can be written as

\begin{eqnarray}
 \intmii dk\pa \left. \int\limits_{-\infty}^{z} d \tilde{z} \right|_{u_f + v\pa > 0}  - \intmii dk\pa\left. \int\limits_{\infty}^{z} d \tilde{z} \right|_{u_f + v\pa < 0}  
\\
=\intmii dk\pa \lp  \int\limits_{-\infty}^{z} d \tilde{z}  + \int\limits_{z}^{\infty} d \tilde{z} \rp
\\
= \intmii dk\pa  \intmii d \tilde{z}
\end{eqnarray} 

(where the initial minus sign is due to the direction of the contour integral) and \eqref{hs_nocauchy} becomes:

\begin{eqnarray}
\label{hs_nocauchy}
\nonumber \hat{h_s} =  
\\
\nonumber \frac{1}{2 \pi \I}  \intmii dk\pa  \intmii d \tilde{z}\frac{1}{ \lp u_f + v\pa^{'} \rp k\pa - \I \gamma^{'} } \exp \lsq - \I k\pa  \lp \tilde{z} - z \rp \rsq 
\\ 
\nonumber \lbr \frac{\I k_y c}{B_0}\lsq \frac{1}{L_n} + \lp \frac{m_s \lp v\pa^{'2} + v\pp^{'2}\rp}{2T_{0s}} -\frac{2}{3} \rp \frac{1}{L_T} \right.\right. \\
\nonumber \left. + 2\frac{u_fv\pa^{'}}{v_{ths}^2} \frac{B_{0t}}{B_{0p}} \frac{1}{L_S} \rsq F_{0s} J_0 \lp \frac{v\pp k\pp}{\OOs} \rp \hat{\varphi} \\
\left. + \frac{e_s}{T_{0s}} \lp J_0 \lp \frac{v\pp k\pp}{\OOs} \rp \pdt{\hat{\varphi}} + u_f \pd{J_0 \lp \frac{v\pp k\pp}{\OOs} \rp\hat{\varphi}}{z}\rp F_{0s} \rbr
\end{eqnarray}

A Boltzmann electron response is now assumed, so that the fluctuating part of the quasineutrality condition is now:

\begin{eqnarray}
\lp 1 + \frac{\tau}{\mathcal{Z}} \rp \frac{q_i n_{0i}}{T_{0i}} \pot = \int d^3 \vct{v^{'}} \gyrav{h_i}{r} 
\end{eqnarray}

which means that:

\begin{eqnarray}
\lp 1 + \frac{\tau}{\mathcal{Z}} \rp \frac{q_i n_{0i}}{T_{0i}} \hat{\pot} = \int d^3 \vct{v^{'}} \Jo{\frac{v\pp k\pp}{\OOs}}\hat{h_i} 
\end{eqnarray}

It can be shown \emph{(cite Ian's paper)?} that the equilibrium distribution function under these circumstances can be written:

\begin{eqnarray}
F_{0i} = \frac{n_{0i}}{\lp \pi v_{thi}^2 \rp^{3/2}} \exp \lsq -\frac{\varepsilon_i}{T_{0i}} \rsq \\ \nonumber
= \frac{n_{0i}}{\lp \pi v_{thi}^2 \rp^{3/2}} \exp \lsq -\frac{v\pp^{'2} + v\pa^{'2}}{v_{thi}^{2}} \rsq + \mathcal{O} \lp \gkeps \rp
\end{eqnarray}
 
Substituting the expression for \(h_i\) into the quasineutrality condition, and using

\begin{eqnarray}
\int d^3 \vct{v^{'}} = \int\limits_{0}^{\infty} d v\pp^{'} v\pp^{'} \int\limits_{-\infty}^{\infty} d v\pa^{'}  \int\limits_{0}^{2 \pi} d \gyr
\end{eqnarray}

the perpendicular velocity integrals are now of the form:

\begin{eqnarray}
\nonumber \Gamma_{00}^{\lp 2n + 1 \rp} = 
\\  
\int\limits_{0}^{\infty} d v\pp^{'} \frac{v\pp^{'\lp 2n + 1\rp}}{v_{thi}^{2n + 2}} \Jo{\frac{v\pp k\pp}{\OOi}} \Jo{\frac{v\pp \tilde{k}\pp}{\OOi}}\exp \lsq -\frac{v\pp^{'2}}{v_{thi}^{2}} \rsq
\end{eqnarray}

where

\begin{eqnarray}
\tilde{k}\pp^2 =  \lp k_x + \frac{\tilde{z}}{l_B} k_y  \rp^2 + k_y^2
\end{eqnarray}.

Defining

\begin{eqnarray}
\rho_i = \frac{v_{thi}}{\OOi}
\end{eqnarray}

\begin{eqnarray}
 \Gamma_{00}^{\lp 2n +1 \rp} = \lp -1 \rp^n \pd[n]{}{\lambda^n}  \\ \nonumber
 \int\limits_{0}^{\infty} d v\pp^{'} \frac{v\pp^{'}}{v_{thi}^2} \Jo{\frac{v\pp}{v_{thi}}k\pp \rho_i} \Jo{\frac{v\pp}{v_{thi}}\tilde{k}\pp \rho_i} \exp \lp -\lambda \frac{v\pp^{'2}}{v_{thi}^{2}} \rp \\ \nonumber
= \lp -1 \rp^n \pd[n]{}{\lambda^n}\frac{1}{\lambda}  \exp \lsq -\frac{\lambda\rho_i^2}{4} \lp k\pp^2 + \tilde{k}\pp^2 \rp \rsq \Io{\frac{\lambda\rho_i^2 k\pp \tilde{k}\pp}{2}}
\end{eqnarray}

In particular the integrals needed are: 

\begin{eqnarray}
\Gamma^{1}_{00} 
\nonumber
\\
= \exp \lsq -\frac{\rho_i^2}{4} \lp k\pp^2 + \tilde{k}\pp^2 \rp \rsq \Io{\frac{\rho_i^2 k\pp \tilde{k}\pp}{2}}
\end{eqnarray}

and 

\begin{eqnarray}
\Gamma^{3}_{00} 
\nonumber
\\
= \Gamma^{1}_{00} \lbr 1   - \frac{\rho_i^2}{4} \lp k\pp^2 + \tilde{k}\pp^2 \rp  + \frac{\rho_i^2 k\pp \tilde{k}\pp}{2}\frac{I_1}{I_0} \rbr
\end{eqnarray}

The parallel velocity integrals are of the form:

\begin{eqnarray}
\frac{1}{\sqrt{\pi}} \intmii d v\pa^{'} \frac{1}{ \lp u_f + v\pa^{'} \rp k\pa - \I \gamma^{'} } \frac{v\pa^{'n}}{v_{thi}^n} \exp \lsq -\frac{v\pa^{'2}}{v_{thi}^2} \rsq
\nonumber \\
=\frac{1}{k\pa\sqrt{\pi}} \intmii d v\pa^{'} \frac{1}{ \frac{v\pa^{'}}{v_{thi}} + \frac{u_f}{v_{thi}}  - \frac{\I \gamma^{'}}{k\pa v_{thi}} } \frac{v\pa^{'n}}{v_{thi}^{n+1}} \exp \lsq -\frac{v\pa^{'2}}{v_{thi}^2} \rsq
\nonumber \\
=\frac{1}{k\pa\sqrt{\pi}} \intmii d t \frac{1}{t - \zeta} t^n \exp \lsq -t^2 \rsq 
\nonumber \\
=\frac{1}{k\pa} Z_n\lp \zeta \rp
\end{eqnarray}

where

\begin{eqnarray}
\zeta  = - \frac{u_f}{v_{thi}}  + \frac{\I \gamma^{'}}{k\pa v_{thi}} 
\end{eqnarray}

and \(Z_0\) is the plasma dispersion function.

The \(\gyr\) integral merely yields a factor of \(2\pi\) since \(\hat{h}_s\) is independent of the gyrophase, and so substituting the expression for \(\hat{h}_s\) into the quasineutrality condition and carrying out the velocity integrals yields:

\begin{eqnarray}
\lp 1 + \frac{\tau}{\mathcal{Z}} \rp \frac{q_i n_{0i}}{T_{0i}} \pot =
\\ \nonumber
\nonumber \frac{2 \pi}{2 \pi \I}\frac{n_{0i}}{\pi}\frac{1}{k\pa}  \intmii dk\pa  \intmii d \tilde{z} \exp \lsq - \I k\pa  \lp \tilde{z} - z \rp \rsq 
\\ 
\nonumber \lbr \frac{\I k_y c}{B_0}\lsq \frac{\Gamma^{1}_{00}Z_0}{L_n} + \lp \Gamma^{1}_{00}Z_2  + \Gamma^{3}_{00}Z_0 -\frac{2}{3} \Gamma^{1}_{00}Z_0 \rp \frac{1}{L_T} \right.\right. \\
\nonumber \left. + 2\frac{u_f}{v_{thi}} \frac{B_{0t}}{B_{0p}} \frac{1}{L_S}  \Gamma^{1}_{00}Z_1 \rsq  \hat{\varphi} \\
\left. + \frac{e_s}{T_{0s}} \lp \gamma^{'}  + \I u_f k\pa \rp \Gamma^{1}_{00}Z_0 \hat{\varphi} \rbr
\end{eqnarray}

\begin{eqnarray}
\nonumber \lp 1 + \frac{\tau}{\mathcal{Z}} \rp \frac{q_i n_{0i}}{T_{0i}} \pot 
\\ 
= \nonumber \frac{1}{\I}\frac{n_{0i}}{\pi}\frac{1}{k\pa}  \intmii dk\pa  \intmii d \tilde{z} \exp \lsq - \I k\pa  \lp \tilde{z} - z \rp \rsq 
\\ 
\nonumber \lbr \frac{\I k_y c}{B_0}\lsq \lp \lp \frac{1}{L_n} - \frac{2}{3}\frac{1}{L_T} \rp \Gamma^{1}_{00} + \frac{1}{L_T}\Gamma^{3}_{00}  \rp Z_0  \right.\right. 
\\ \nonumber
\left. +  \frac{1}{L_T}\Gamma^{1}_{00}Z_2    + 2\frac{u_f}{v_{thi}} \frac{B_{0t}}{B_{0p}} \frac{1}{L_S}  \Gamma^{1}_{00}Z_1 \rsq  \hat{\varphi} \\
\left. - \frac{\I e_s k\pa v_{thi}}{T_{0s}}  \zeta \Gamma^{1}_{00}Z_0 \hat{\pot} \rbr
\end{eqnarray}

Normalizing \(\pot\) to \(e_i / T_{0i}\) and cancelling factors of \(\I\):  

\begin{eqnarray}
\lp 1 + \frac{\tau}{\mathcal{Z}} \rp  \pot =
\\ \nonumber
\nonumber \frac{1}{\pi}\frac{1}{k\pa}  \intmii dk\pa  \intmii d \tilde{z} \exp \lsq - \I k\pa  \lp \tilde{z} - z \rp \rsq 
\\ 
\nonumber \lbr \frac{k_y c T_{0i}}{B_0 e_i}\lsq \lp \lp \frac{1}{L_n} - \frac{2}{3}\frac{1}{L_T} \rp \Gamma^{1}_{00} + \frac{1}{L_T}\Gamma^{3}_{00}  \rp Z_0  \right.\right. 
\\ \nonumber
\left. +  \frac{1}{L_T}\Gamma^{1}_{00}Z_2    + 2\frac{u_f}{v_{thi}} \frac{B_{0t}}{B_{0p}} \frac{1}{L_S}  \Gamma^{1}_{00}Z_1 \rsq  \hat{\varphi} \\
\left. -  k\pa v_{thi}  \zeta \Gamma^{1}_{00}Z_0 \hat{\pot} \rbr
\end{eqnarray}

Lastly note that

\begin{eqnarray}
\frac{k_y c T_{0i}}{B_0 e_i} = \frac{k_y c m_i v_{thi}^2}{2 B_0 e_i} = \frac{k_y v_{thi}^2}{2 \OOi} = \frac{k_y \rho_i v_{thi}}{2}
\end{eqnarray}

So that: 

\begin{eqnarray}
\lp 1 + \frac{\tau}{\mathcal{Z}} \rp  \pot =
\\ \nonumber
\nonumber \frac{1}{\pi}  \intmii dk\pa  \intmii d \tilde{z} \exp \lsq - \I k\pa  \lp \tilde{z} - z \rp \rsq 
\\ 
\nonumber \frac{k_y \rho_i v_{thi}}{2k\pa}\lsq \lp \lp \frac{1}{L_n} - \frac{2}{3}\frac{1}{L_T} - \frac{2k\pa}{k_y \rho_i} \zeta \rp \Gamma^{1}_{00} + \frac{1}{L_T}\Gamma^{3}_{00}  \rp Z_0  \right. 
\\ \nonumber
\left. +  \frac{1}{L_T}\Gamma^{1}_{00}Z_2    + 2\frac{u_f}{v_{thi}} \frac{B_{0t}}{B_{0p}} \frac{1}{L_S}  \Gamma^{1}_{00}Z_1 \rsq  \hat{\varphi}
\end{eqnarray}

\chapter{A New Implementation of Flow Shear in AstroGK}
\chapter{A Note on Geometry}
\label{geometryapp}
